# Supplementary material for: FOAL: Fine-grained Contrastive Learning for Cross-domain Aspect Sentiment Triplet Extraction
Source: arXiv:2311.10373 source file (2023-11-17)
Supplement: Supplementary file 1 [file 0_exp.tex]

\section{Experiments}

\subsection{Training Details}
\label{sec:train-detail}
\XT{paraphrase this paragraph}
We utilize the pre-trained model provided by \href{https://huggingface.co/}{HuaggingFace} and run all the experiments on NVIDIA A100 GPU with PyTorch.
For adversarial training, we follow the implementation in \citet{ganin2016domain}. One parameter for this method is $\alpha$, the ratio of training the generator to the discriminator. We search $\alpha$ in $\{1, 3, 5, 7, 10, 30, 50\}$ and $\{1, 10, 50, 100, 500, 700, 1000, 1500\}$ for Span-ASTE + AT and BMRC + AT, respectively. For each value, we conduct experiments with 5 random seeds and set $\alpha$ by the F1 score on the development set. We set $\alpha=5$  for Span-ASTE + AT and $\alpha=1000$ for BMRC + AT. The parameter search costs about 1000 GPU hours.

\subsection{Hyper-parameter Analysis}
We have three hyper-parameters in this study, i.e., the sharpening temperature $\tau$, the pseudo-label threshold $t$, and the weight parameter $\lambda$. We tune all the hyper-parameters based on the model performance on the evaluation set. Results are shown in Figure \ref{fig:hyper}. We finally set $\tau=20, t=0.93, \lambda=0.3$ for all transfer pairs.

\subsection{Experiments For Adversarial Training}
We search the hyper-parameter $\alpha$ for adversarial learning on the evaluation set.
Detailed experiment results are shown in Table \ref{tab:span-at} and Table \ref{tab:bmrc-at}. We can observe that adversarial training is parameter-sensitive. And the adversarial training is not adequate for the cross-domain ASTE task.
\input{tables/span_at.tex}
\input{tables/bmrc_at.tex}
